# Supplementary material for: Dismantling Pathological Shortcuts: A Causal Framework for Faithful LVLM Decoding
Source: arXiv:2606.27596 source file (2026-06-25)
Supplement: Supplementary file 1 [file Appendix_MME_Detailed.tex]

% \begin{table}[t]
% \centering
% \caption{\textbf{Detailed results on MME.} All methods adopt the same sampling decoding strategy.}
% \vspace{-0.35em}
% \small
% \setlength{\tabcolsep}{8pt} % 调整列间距
% \renewcommand{\arraystretch}{1.2} % 调整行间距，使表格更像图片那样舒展

% \begin{tabular}{llccccc} % 移除竖线 |，改为纯对齐
% \toprule
% \multirow{2}{*}{\textbf{Model}} & \multirow{2}{*}{\textbf{Method}} &
% \multicolumn{2}{c}{\textbf{Object-level}} &
% \multicolumn{2}{c}{\textbf{Attribute-level}} &
% \multirow{2}{*}{\textbf{Total Score} $\uparrow$} \\
% \cmidrule(lr){3-4} \cmidrule(lr){5-6} % 局部横线，(lr)让线条左右留白，区分度更好
% & & Existence $\uparrow$ & Count $\uparrow$ &
% Position $\uparrow$ & Color $\uparrow$ & \\
% \midrule

% % 第一组：LLaVA-1.5
% \multirow{4}{*}{\textbf{LLaVA-1.5}}
% & Regular  & 171.7 & 120.8 & 112.6 & 151.0 & 556.1 \\
% & DoLa     & 173.2 & 122.4 & 115.2 & 152.8 & 563.6 \\
% & VCD      & 174.4 & 124.1 & 119.4 & 153.6 & 571.5 \\

% & \textbf{Ours} & \textbf{180.5} & \textbf{130.7} & \textbf{123.8} & \textbf{154.5} & \textbf{589.5} \\
% \midrule

% % 第二组：InstructBLIP
% \multirow{4}{*}{\textbf{InstructBLIP}}
% & Regular  & 171.7 & 120.8 & 112.6 & 151.0 & 556.1 \\
% & DoLa     & 173.2 & 122.4 & 115.2 & 152.8 & 563.6 \\
% & VCD      & 174.4 & 124.1 & 119.4 & 153.6 & 571.5 \\

% & \textbf{Ours} & \textbf{180.5} & \textbf{130.7} & \textbf{123.8} & \textbf{154.5} & \textbf{589.5} \\
% \midrule

% % 第三组：Shikra
% \multirow{4}{*}{\textbf{Shikra}}
% & Regular  & 171.7 & 120.8 & 112.6 & 151.0 & 556.1 \\
% & DoLa     & 173.2 & 122.4 & 115.2 & 152.8 & 563.6 \\
% & VCD      & 174.4 & 124.1 & 119.4 & 153.6 & 571.5 \\

% & \textbf{Ours} & \textbf{180.5} & \textbf{130.7} & \textbf{123.8} & \textbf{154.5} & \textbf{589.5} \\
% \bottomrule
% \end{tabular}

% \label{tab:mme_detail}
% \end{table}
