# Supplementary material for: Dismantling Pathological Shortcuts: A Causal Framework for Faithful LVLM Decoding
Source: arXiv:2606.27596 source file (2026-06-25)
Supplement: Supplementary file 2 [file Appendix_POPE_Detailed.tex]

% % \documentclass{article}
% % % 所有必需包（按顺序加载）
% % \usepackage{adjustbox}    % 缩放表格
% % \usepackage{booktabs}     % 表格线
% % \usepackage{array}        % 表格底层增强
% % \usepackage{multirow}     % 多行合并
% % \usepackage{amsmath}      % 数学符号
% % \usepackage{caption}      % 标题格式（可选，优化caption显示）

% % \begin{document}

% % 表格前无任何多余代码，避免上下文干扰
% \begin{table*}[t]
% \centering
% % 修正 adjustbox 语法 + 表格列格式
% \begin{adjustbox}{max width=\textwidth}
% \begin{tabular*}{\textwidth}{@{\extracolsep{\fill}} c l l cc cc cc @{}}
% \toprule
% \multirow{2}{*}{\textbf{Dataset}} &
% \multirow{2}{*}{\textbf{Setting}} &
% \multirow{2}{*}{\textbf{Method}} &
% \multicolumn{2}{c}{\textbf{LLaVA-v1.5}} &
% \multicolumn{2}{c}{\textbf{InstructBlip}} &
% \multicolumn{2}{c}{\textbf{Shikra}} \\
% & & & Acc & F1 & Acc & F1 & Acc & F1 \\
% \midrule

% % ================= MS-COCO =================
% \multirow{15}{*}{MS-COCO} & \multirow{5}{*}{Random} & Sampling   & 83.8 & 84.2 & 84.9 & 82.9 & 84.4 & 82.3 \\
% & & VCD                & 85.0 & 84.2 & 85.5 & 83.6 & 86.0 & 84.3 \\
% & & ICD               & 86.1 & 85.0 & 85.3 & 83.4 & 85.5 & 83.6 \\
% & & AvisC              & 82.3 & 83.5 & 82.9 & 80.0 & 85.2 & 82.8 \\
% & & \M~(Ours)         & \textbf{89.2} & \textbf{89.1} & \textbf{86.0} & \textbf{84.1} & \textbf{86.6} & \textbf{84.8} \\
% \cmidrule(lr){2-3}\cmidrule(lr){4-9}

% & \multirow{5}{*}{popular} & Sampling & 82.0 & 82.6 & 84.0 & 81.9 & 83.2 & 81.5 \\
% & & VCD                  & 82.1 & 83.2 & 84.9 & 83.6 & 84.5 & 82.9 \\
% & & ICD                 & 82.8 & 84.1 & 84.2 & 82.7 & 84.20 & 82.4 \\
% & & AvisC                & 78.2 & 80.5 & 82.8 & 80.1 & 83.9 & 81.6 \\
% & & \M~(Ours)           & \textbf{85.7} & \textbf{86.1} & \textbf{85.6} & \textbf{83.7} & \textbf{85.5} & \textbf{83.8} \\
% \cmidrule(lr){2-3}\cmidrule(lr){4-9}

% & \multirow{5}{*}{adversarial} & sampling & 75.8 & 78.1 & 82.1 & 80.2 & 79.5 & 78.1 \\
% & & VCD                      & 76.3 & 78.7 & 84.0 & 82.0 & 80.9 & 79.7 \\
% & & ICD                     & 77.1 & 78.9 & 83.2 & 80.8 & 80.6 & 79.2 \\
% & & AvisC                    & 74.2 & 77.7 & 81.2 & 78.5 & 81.8 & 80.2 \\
% & & MoD (Ours)               & \textbf{79.7} & \textbf{81.3} & \textbf{84.0} & \textbf{82.3} & \textbf{82.4} & \textbf{81.0} \\
% \midrule

% % ================= A-OKVQA =================
% \multirow{15}{*}{A-OKVQA} & \multirow{5}{*}{random} & sampling & 81.8 & 83.5 & 86.8 & 85.8 & 83.8 & 83.0 \\
% & & VCD                                 & 81.2 & 83.2 & 87.4 & 86.6 & 84.8 & 83.9 \\
% & & ICD                                & 82.9 & 84.6 & 87.1 & 85.9 & 85.3 & 84.3 \\
% & & AvisC                               & 79.1 & 82.1 & 84.7 & 83.0 & 85.8 & 84.4 \\
% & & MoD (Ours)                          & \textbf{86.5} & \textbf{87.5} & \textbf{87.8} & \textbf{86.9} & \textbf{86.4} & \textbf{85.6} \\
% \cmidrule(lr){2-3}\cmidrule(lr){4-9}

% & \multirow{5}{*}{popular} & sampling & 75.3 & 78.7 & 85.6 & 84.7 & 81.4 & 80.8 \\
% & & VCD                                 & 74.7 & 78.5 & 86.3 & 85.1 & 81.5 & 81.2 \\
% & & ICD                                & 75.8 & 79.4 & 85.9 & 84.6 & 82.2 & 81.6 \\
% & & AvisC                               & 71.8 & 77.2 & 83.9 & 82.4 & 83.9 & 82.8 \\
% & & MoD (Ours)                          & \textbf{79.5} & \textbf{82.2} & \textbf{86.5} & \textbf{85.6} & \textbf{84.2} & \textbf{83.6} \\
% \cmidrule(lr){2-3}\cmidrule(lr){4-9}

% & \multirow{5}{*}{adversarial} & sampling & 67.4 & 73.7 & 80.4 & 80.5 & 73.2 & 74.5 \\
% & & VCD                                   & 68.1 & 74.6 & 80.7 & 80.8 & 74.7 & 76.0 \\
% & & ICD                                  & 68.3 & 74.6 & 80.5 & 80.4 & 74.6 & 75.7 \\
% & & AvisC                                 & 64.4 & 73.0 & 78.1 & 77.3 & 75.6 & 76.6 \\
% & & MoD (Ours)                            & \textbf{69.1} & \textbf{75.4} & \textbf{81.0} & \textbf{80.9} & \textbf{75.7} & \textbf{76.9} \\
% \midrule

% % ================= GQA =================
% \multirow{15}{*}{GQA} & \multirow{5}{*}{random} & sampling & 81.6 & 83.5 & 81.3 & 79.2 & 83.1 & 82.5 \\
% & & VCD                                  & 82.2 & 84.1 & 82.0 & 80.5 & 84.0 & 83.4 \\
% & & ICD                                 & 83.3 & 84.5 & 82.4 & 79.7 & 84.3 & 83.5 \\
% & & AvisC                                & 79.0 & 82.2 & 80.5 & 77.8 & 84.9 & 83.4 \\
% & & MoD (Ours)                           & \textbf{86.2} & \textbf{87.4} & \textbf{83.8} & \textbf{82.3} & \textbf{86.2} & \textbf{85.5} \\
% \cmidrule(lr){2-3}\cmidrule(lr){4-9}

% & \multirow{5}{*}{popular} & sampling & 73.1 & 77.5 & 75.9 & 74.9 & 78.5 & 78.5 \\
% & & VCD                                  & 71.5 & 76.8 & 75.9 & 75.6 & 78.2 & 78.6 \\
% & & ICD                                 & 72.3 & 77.1 & 76.8 & 77.0 & 78.8 & 78.9 \\
% & & AvisC                                & 67.4 & 74.8 & 74.2 & 72.3 & 80.5 & 79.5 \\
% & & MoD (Ours)                           & \textbf{74.0} & \textbf{78.6} & \textbf{79.8} & \textbf{78.9} & \textbf{81.1} & \textbf{81.1} \\
% \cmidrule(lr){2-3}\cmidrule(lr){4-9}

% & \multirow{5}{*}{adversarial} & sampling & 68.0 & 74.5 & 75.5 & 74.4 & 73.3 & 74.5 \\
% & & VCD                                    & 67.6 & 74.5 & 76.7 & 76.2 & 74.2 & 75.6 \\
% & & ICD                                   & 67.2 & 74.0 & 77.1 & 76.7 & 74.2 & 75.4 \\
% & & AvisC                                  & 64.1 & 72.9 & 75.5 & 73.4 & 75.8 & 75.9 \\
% & & MoD (Ours)                             & \textbf{68.7} & \textbf{75.3} & \textbf{78.9} & \textbf{78.1} & \textbf{76.0} & \textbf{77.2} \\
% \bottomrule
% \end{tabular*}
% \end{adjustbox}
% \vspace{-0.35em}
% \caption{\textbf{Detailed results on POPE under sampling decoding.} ``Acc'' and ``F1'' denote Accuracy and F1 score, respectively.}
% \label{tab:pope_sampling_detail}
% \vspace{-0.5em}
% \end{table*}

% % \end{document}
